# Supplementary material for: Superfluidity of indirect momentum space dark dipolar excitons in a double layer with massive anisotropic tilted semi-Dirac bands
Source: arXiv:2401.12154 source file (2024-01-22)
Supplement: Supplementary file 1 [file VSupplementary_materials.tex]

\documentclass[preprintnumbers,amsmath,amssymb,10pt]{revtex4}

\setlength{\arrayrulewidth}{0.2mm}
\setlength{\tabcolsep}{18pt}

\usepackage{graphicx}
\usepackage{color}
\usepackage{float}
\usepackage{amsmath}
\usepackage{appendix}

\thispagestyle{empty}
\begin{document}

\title{Supplemental information for Superfluidity of indirect momentum space dark dipolar excitons in a double layer with massive anisotropic tilted semi-Dirac bands}

\affiliation{$^{1}$Physics Department, New York City College
of Technology,          The City University of New York, \\
300 Jay Street,  Brooklyn, NY 11201, USA \\
 $^{2}$The Graduate School and University Center, The
City University of New York, \\
365 Fifth Avenue,  New York, NY 10016, USA\\
 $^{3}$Department of Physics and Astronomy, Hunter College of The City University of New York, 695 Park Avenue, \\
New York, NY 10065, USA\\
$^{4}$Donostia International Physics Center (DIPC), P de Manuel Lardizabal, 4, 20018 San Sebastian, Basque Country, Spain }

\date{\today}

\maketitle

\section{In-plane gyration radius of dipolar exciton}

We consider the layers to be separated by $h$-BN insulating layers. For this insulator $\varepsilon_d$ = 4.89 is the effective dielectric constant, defined as $ \varepsilon_d = \sqrt{\varepsilon^{\perp}} \sqrt{\varepsilon^{\parallel}} $, where $ \sqrt{\varepsilon^{\perp}} = 6.71 $ and $ \sqrt{\varepsilon^{\parallel}} = 3.56 $ are components of the dielectric tensor for $h$-BN. Since the thickness of a $h$-BN monolayer is given by $c_1 = 3.33 $ \r{A} the interlayer separation $D$ is given by $D = N_L c_1 $. while for the SiO$_2$ barrier we substitute the dielectric constant $\varepsilon_d = 4.50$. For choice of dielectric, it is preferable to use h-BN since it reduces the degradation of the heterostructure and the PL linewidth. One can obtain the square of the in-plane gyration radius $r_X$ of a dipolar exciton, which is the average squared projection of the electron-hole separation onto the plane of a monolayer \cite{Butov}, as

\begin{eqnarray}
r_X^2 = \int \phi_{00}^{*}(x,y) r^2 \phi_{00}(x,y) d^2r = \frac{a_x^2 + a_y^2}{2}
\label{gyrationRadius}
\end{eqnarray}
\noindent
We emphasize that the Taylor series expansion of the electron-hole attraction to first order in $(r/D)^2$ presented in Eq.(B.1) is valid if the inequality $ \langle r^2 \rangle = r_X^2 =(a_x^2 + a_y^2)/2 \ll D^2 $ is satisfied, where $a_x$ and $a_y$ are defined above. Consequently we find that the $ \hbar/(2\sqrt{2 \mu_0 \gamma}) \ll D^2 $. The latter inequality holds for $D \gg D_0$. For the Coulomb potential $D_0 = \hbar^2 \varepsilon_d / (4 ke^2 \mu_0)$.

\section{Collective excitations calculations}

In this section we provide supplementary materials for Section V.A.
The results in this section are adapted from known formulations and
standard procedures. \noindent Using the procedure {
presented in
\cite{SuperfluidDipolar,HighTempSuperOleg,nanomatGabriel},} the
interaction parameters for the exciton-exciton interaction in very
dilute system could be obtained assuming the exciton-exciton
dipole-dipole repulsion exists only at distances between excitons
greater than the distances between exciton to the classical turning
point. The distance between two excitons cannot be less than this
distance, which is determined by the conditions reflecting the fact
that the energy of two excitons cannot exceed double the chemical
potential of the system \cite{LifPit}
\begin{align}
2\mathcal{A}_A + U(R_{0AA}) &= 2\mu_A\\
2\mathcal{A}_B + U(R_{0BB}) &= 2\mu_B\\
\mathcal{A} + \mathcal{B} + U(R_{0AB}) &= \mu_A + \mu_B
\label{chemicalPotExceed}
\end{align}
\noindent
where $R_{0AA}$, $R_{0BB}$, and $R_{0AB}$ are distances between two excitons at the classical turning point for two $A$ excitons, two $B$ excitons, and one $A$ and one $B$ exciton, correspondingly. In thermodynamic equilibrium, the chemical potentials of $A$ and $B$ excitons are equal. From Eq.~(\ref{chemicalPotExceed}) we can obtain

\begin{align}
R_{0AA} &= \left(\frac{ke^2D^2}{2\epsilon_d(\mu_A -\mathcal{A}_A)}\right)^{1/3} \\
R_{0BB} &= \left(\frac{ke^2D^2}{2\epsilon_d(\mu_B -\mathcal{A}_B)}\right)^{1/3} \\
R_{0AB} &= \left(\frac{ke^2D^2}{\epsilon_d (\mu_A + \mu_B -\mathcal{A}_A-\mathcal{A}_B)}\right)^{1/3}
\label{RO}
\end{align}
\noindent
The Hamiltonian $\hat{H}$ of the 2D $A$ and $B$ interacting excitons is given by

\begin{equation}
\hat{H} = \hat{H}_A +\hat{H}_B  +\hat{H}_I \  ,
\label{Hamiltonian}
\end{equation}
\noindent
where $\hat{H}_A(B)$ are the Hamiltonians of $A(B)$ excitons given by

\begin{equation}
\hat{H}_{A(B)} = \sum_{\textbf{P}} E_{A(B)}(P,\Theta) a^{\dag}_{\textbf{P}A(B)} a_{\textbf{P}A(B)} + \frac{g_{AA(BB)}}{2S} \sum_{\textbf{PLM}} \varepsilon_0(P,\Theta) a^{\dag}_{\textbf{P}A(B)} a^{\dag}_{\textbf{L}A(B)} a_{\textbf{M}A(B)}  a_{\textbf{P+L-M}A(B)}
\label{HamiltonianAB}
\end{equation}
\noindent
and $\hat{H}_I$ is the Hamiltonian of the interaction between $A$ and $B$ excitons given by

\begin{equation}
\hat{H}_{I} = \frac{g_{AB}}{S} \sum_{\textbf{PLM}} a^{\dag}_{\textbf{P}A} a^{\dag}_{\textbf{L}B} a_{\textbf{M}B} a_{\textbf{P+L-M}A}    \  ,
\label{HamiltonianI}
\end{equation}
\noindent
where $a^{\dag}_{P A(B)}$ and $a_{P A(B)}$ are Bose creation and annihilation operators for $A(B)$ excitons with momentum \textbf{P}, $S$ is the area of the system, $\varepsilon(P,\Theta)$ is the angular-dependent energy spectrum of non-interacting excitons, $E_{A(B)} (P,\Theta) = \varepsilon_{(0)A(B)} (P,\Theta) + \mathcal{A}_{A(B)}$ is the energy spectrum of noninteracting $A (B)$ excitons, where $\mathcal{A}_{A(B)}$ is the constant, which depends on $A(B)$ binding energy and the gap formed by a spin-orbit coupling gap for the $A(B)$ exciton, $g_{AA(BB)}$ and $g_{AB}$ are the interaction constants for the interaction between two $A$ excitons, two $B$ excitons, and for the interaction between $A$ and $B$ excitons. It is worthy of note that the energy spectrum of the center of mass of an electron-hole pair $\varepsilon_{0 A(B)}(\textbf{P})$ may be expressed as
\begin{equation}
\varepsilon_{0 A(B)}(\textbf{P}) = \frac{P^2_x}{2 M_{xA(B)}} + \frac{P^2_y}{2 M_{yA(B)}}
\label{Energy_Naught}
\end{equation}
\noindent
where $M_x = m^e_x + m^h_x$, and $M_y = m^e_y + m^h_y$ are the effective exciton masses, relating to the motion of an electron-hole center of mass in the $x$ and $y$ directions, respectively. Substituting the polar coordinate for the momentum $P_x = P \cos \Theta$ and $P_y = P \sin \Theta$ into the above equation Eq.~(\ref{Energy_Naught}), we obtain

\begin{equation}
\varepsilon_{0 A(B)}({p},\Theta) = \frac{P^2}{2 M_0 (\Theta)}
\label{Energy_Naught_cond}
\end{equation}
\noindent
where $M_{0 A(B)}(\Theta)$ is the effective angle dependant exciton mass given by

\begin{equation}
M_{0 A(B)}(\Theta) = \left[\frac{\cos^2 \Theta}{M_{xA(B)}} +\frac{\sin^2 \Theta}{M_{yA(B)}} \right]^{-1}
\label{Mass_Theta}
\end{equation}

We can also obtain the interaction constants for the exciton-exciton interaction using the standard procedure outlined in \cite{OKKL}

\begin{eqnarray}
g_{AA} = \frac{2\pi ke^2D^2}{\epsilon_d R_{0AA}}, \hspace{0.6cm}
g_{BB} = \frac{2\pi ke^2D^2}{\epsilon_d R_{0BB}}, \hspace{0.6cm}
g_{AB} = \frac{2\pi ke^2D^2}{\epsilon_d R_{0AB}}
\label{g}
\end{eqnarray}

\noindent
From Eq.~(\ref{Hamiltonian})-(\ref{HamiltonianI}), we obtain

\begin{equation}
\hat{H}_0 - \mu \hat{N} = S \left[(\mathcal{A}_A - \mu_A)n_A +(\mathcal{A}_B - \mu_B)n_B + \frac{g_{AA} n^2_A}{2}+ \frac{g_{BB} n^2_B}{2}+g_{AB}n_An_B\right] \  ,
\label{minimizePot}
\end{equation}
\noindent
where $\mu_A$ and $\mu_B$ are the chemical potential for $A$ and $B$ excitons, respectively, of the weakly interacting Bose gas of excitons within the Bogoliubov approximation, and $n_A$ and $n_B$ are the 2D concentration of $A$ and $B$ excitons, respectively. The minimization of $\hat{H}_0 - \mu \hat{N}$ with respect to the number of A excitons $N_A = S n_A$ and B excitons $N_B = Sn_B$ yields the following

\begin{align}
\mu_A - \mathcal{A}_A &= g_{AA}n_{A} + g_{AB}n_B \\
\mu_B - \mathcal{A}_B &= g_{BB}n_{B} + g_{AB}n_A \\
\mu_A + \mu_B - \mathcal{A}_A - \mathcal{A}_B &= g_{AA}n_{A} +g_{BB}n_{B}+ g_{AB}n  \  ,
\label{chemicalPot}
\end{align}
\noindent
where $n = n_A + n_B$ is the 2D concentration of excitons. Combining Eqn.~(36) and Eqn.~(\ref{chemicalPot}) one obtains the following system of three cubic equations for the interaction constants $g_{AA}, g_{BB}, g_{AB}$:

\begin{flalign}
&g^3_{AA} - 2\mathcal{B}n_{A}g_{AA} - 2\mathcal{B}n_{B}g_{AB} = 0 \\
&g^3_{BB} - 2\mathcal{B}n_{B}g_{BB} - 2\mathcal{B}n_{AX}g_{AB} = 0 \\
&2g^3_{AB} = g^3_{AA} +g^3_{BB}  \  ,
\label{chemicalPotCubic}
\end{flalign}
\noindent
where $\mathcal{B}$ is defined as

\begin{equation}
\mathcal{B} = \frac{(2\pi)^3(ke^2D^2)^2}{\epsilon^3_d}
\label{mathB}
\end{equation}
\noindent
If the interaction constants for the exciton-exciton interaction are negative, the spectrum of collective excitations at small momenta is imaginary which reflects the instability of the excitonic ground state. The system of equations in Eq.~(\ref{chemicalPotCubic}) has all positive and real roots only if $g_{AA} = g_{BB} = g_{AB} = g$. Substituting this condition above, we obtain

\begin{align}
g^3 - 2 \mathcal{B}(n_A + n_B)g = 0
\label{chemicalPotCubicG}
\end{align}
\noindent
Using $n = n_A + n_B$, we get the following expression for g:

\begin{equation}
g = \sqrt{2 \mathcal{B}n}
\label{cubicG}
\end{equation}
\noindent
Substituting Eq.~(\ref{mathB}) into Eq.~(\ref{cubicG}) we obtain $g$ as

\begin{equation}
g = \frac{4\pi k e^2 D^2 \sqrt{\pi n}}{\epsilon_d}
\label{constantG}
\end{equation}
\noindent
Using the notation below,

\begin{flalign}
&G_{AA} = g_{AA}n_{A} =g n_A \\
&G_{BB} = g_{BB}n_{B} =g n_B \\
&G_{AB} = g_{AB}\sqrt{n_{A} n_B} =g \sqrt{n_A n_B} \\
&\omega_A(P, \Theta) = \sqrt{\varepsilon^2_{(0)A}(P,\Theta) + 2 G_{AA}\varepsilon_{(0)A}(P,\Theta)} \\
&\omega_B(P, \Theta) = \sqrt{\varepsilon^2_{(0)B}(P,\Theta) + 2 G_{BB}\varepsilon_{(0)B}(P,\Theta)}
\label{notationExc}
\end{flalign}
\noindent
we obtain two modes of the spectrum of the spectrum of Bose collective excitations $\varepsilon_j(p,\Theta)$ in the Bogoliubov approximation for two-component weakly interacting Bose gas

\begin{equation}
\varepsilon_j(P,\Theta) = \sqrt{\frac{\omega^2_A(P,\Theta)+\omega^2_B(P,\Theta) +(-1)^{j-1}\sqrt{\left[\omega^2_A(P,\Theta) -\omega^2_B(P,\Theta)\right]^2 + \left(4G_{AB}\right)^2\varepsilon_{(0)A}(P,\Theta)\varepsilon_{(0)B}(P,\Theta)}}{2}}  \  ,
\label{spectrumJ}
\end{equation}
\noindent
where $j = 1,2$. We can note that $G_{AB}^2 = G_{AA}G_{BB}$. We consider the dilute limit for gases of electrons and holes in parallel layers spatially separated by a dielectric, when $n_A a_{BA}^2$ $\ll$ 1 and $n_B a_{BB}^2 \ll 1$, where $n_{A(B)}$ and $a_{BA(B)}$ are the concentrations and effective exciton Bohr radii for $A (B)$ excitons, correspondingly.

% Make a note about the fact that C exciton production can be restricted by the use of different polarizations of light. A paper we have references this

\end{document}
